# Supplementary material for: Accurate Action Recommendation for Smart Home via Two-Level Encoders and Commonsense Knowledge
Source: arXiv:2208.06089 source file (2022-08-12)
Supplement: Supplementary file 1 [file 060appendix.tex]

\section*{Appendix}
\label{sec:appendix}
